# Supplementary material for: Spontaneous tilt of single-clamped thermal elastic sheets
Source: arXiv:2104.11733 ancillary file (2021-04-29)
Supplement: Supplementary file 1 [file Tilt_SI.pdf]

**Supplementary Material for:  
Spontaneous tilt of single-clamped thermal elastic sheets**

Zhitao Chen,<sup>1</sup> Duanduan Wan,<sup>2</sup> and Mark J. Bowick<sup>3, \*</sup>

<sup>1</sup>*Department of Physics, University of California Santa Barbara, Santa Barbara, California 93106, USA*

<sup>2</sup>*School of Physics and Technology, Wuhan University, Wuhan 430072, China*

<sup>3</sup>*Kavli Institute for Theoretical Physics, University of California Santa Barbara, Santa Barbara, California 93106, USA*

**This PDF includes:**

Captions for Movies S1 to S4

Materials and Methods

Figures S1 to S3

References

**Other Supplementary Material for this manuscript includes the following:**

Movies S1 to S4 (.mpg)

## I. CAPTIONS FOR MOVIES S1 TO S4

Movies S1 to S4 show the vibration of an elastic sheet with zero-temperature length  $L_0 = 20a$  and aspect ratio  $\alpha = W_0/L_0 \approx 5$ . The sheet is clamped along one edge at its zero-temperature width  $W_0$  (colored in pink). The temperatures are  $kT = 0.1, 0.8, 0.5$  eV. The exhibits a horizontal phase and a tilt phase. In the tilt phase it also flips between the up and the down states with the same mean tilt angle. Movie S3 is taken over a longer time interval to demonstrate several inversions. Movie S4 uses the same parameters as Movie S3, but shows a side view. In all the movies there is a fixed horizontal reference plane (blue) corresponding to the zero-temperature ground state. The movie files are:

Movie\_S1.flat.mpg  
 Movie\_S2.tilt.mpg  
 Movie\_S3.flip.mpg  
 Movie\_S4.flip\_sideview.mpg

## II. MOLECULAR DYNAMICS SIMULATION

In thin sheet elasticity theory the free energy is given by the sum of stretching and bending terms [1, 2]:  $F_{el} = F_s + F_b$ . For a discrete triangulation the stretching energy is [3–5]

$$F_s = \frac{\varepsilon}{2} \sum_{\langle ij \rangle} (|\mathbf{r}_i - \mathbf{r}_j| - a)^2, \quad (\text{S1})$$

and the bending energy is

$$F_b = \frac{\tilde{\kappa}}{2} \sum_{\langle IJ \rangle} (\hat{\mathbf{n}}_I - \hat{\mathbf{n}}_J)^2, \quad (\text{S2})$$

where  $\varepsilon$  is the discrete spring constant,  $a$  is the equilibrium spring length and  $\tilde{\kappa}$  is the discrete bending modulus. As usual  $\langle ij \rangle$  denotes pairs of nearest-neighbor vertices, with positions  $\mathbf{r}_i$  in the 3D Euclidean embedding space and  $\langle IJ \rangle$  denotes pairs of triangular plaquettes sharing a common edge, with  $\hat{\mathbf{n}}_I$  being their unit normals. The corresponding continuum moduli are  $Y = 2\varepsilon/\sqrt{3}$ ,  $\kappa = \sqrt{3}\tilde{\kappa}/2$  and Poisson ratio  $\nu = 1/3$  [3–5]. The lattice constant  $a$  can be taken as the distance between neighboring hexagons when describing the dual honeycomb lattice applicable to graphene. This discretized model has been used to study a wide variety of 2D elastic membranes (see Ref. [6]). With graphene as a concrete example, we set the equilibrium spring length  $a$  to be  $\sqrt{3}a_0$ , where  $a_0 = 1.42 \text{ \AA}$  is the carbon-carbon bond length in graphene – thus  $a \approx 2.46 \text{ \AA}$ , where we again note that the triangular lattice we employ is the dual of graphene’s honeycomb lattice. To give the correct graphene density we take the mass of every vertex to be  $m = 2m_C \approx 4 \times 10^{-26} \text{ kg}$ , where  $m_C$  is the mass of a carbon atom. We choose  $a$  and  $m$  as our units of length and mass and set  $a = 1$  and  $m = 1$  in all simulations. Fig. 1(a) of the main text displays the initial, zero-temperature flat configuration of the membrane in the  $x - y$  plane, with  $n_1 = 21$  vertices in the short ( $x$ ) direction and  $n_2 = 117$  vertices staggered along the long ( $y$ ) direction ( $L_0 \approx 20a \approx 50 \text{ \AA}$  and  $W_0 = 58\sqrt{3}a \approx 100 \text{ \AA}$ ). There are 2399 vertices in total. We perform MD simulations using both the HOOMD-blue [7, 8] and the LAMMPS software packages [9] and find consistent results. We choose  $E_0 = 1 \text{ eV}$  as the unit of energy in all simulations. The elastic free energy is calculated as the sum of the stretching and bending energies given in Eqs. (S1) and (S2), with bare elastic parameters  $\kappa = 1.2 \text{ eV}$  [10, 11] and  $Y = 20 \text{ eV/\AA}^2$  [12, 13] for graphene. The discrete parameters  $\varepsilon$  and  $\tilde{\kappa}$  follow from the relations above. After giving the free vertices a small random out-of-plane displacement, we update their positions in the constant temperature (NVT) ensemble. The simulation unit of time thus corresponds to a real time  $t_0 = \sqrt{ma^2/E_0} \approx 0.12 \text{ ps}$ . Finally we set the integration timestep to be 0.005. Every simulation timestep  $\tau$  thus corresponds to a real time  $\tau = 0.005 t_0 \approx 0.6 \text{ fs}$ . Every simulation run consists of  $10^7$  time steps in total, with the first  $5 \times 10^6$  time steps ensuring equilibration. For data analysis we discard one configuration every  $10^4$  time steps in the second  $5 \times 10^6$  timesteps.

## III. FINITE ELEMENT SIMULATION

We perform a finite element (FE) simulation using the FEniCS package [14] to obtain the distribution of the in-plane stress field. As an example, we take a rectangular sheet with an aspect ratio  $\alpha = 2$  and a strain  $\epsilon = 0.05$  at  $x = 0$ . Fig. 4 in the main text shows  $\sigma_{xx}$  and  $\sigma_{yy}$ . These are reproduced here in Fig. S1, along with  $\sigma_{xy}$ . The “crescent moon” region of high  $\sigma_{xx}$  and  $\sigma_{yy}$

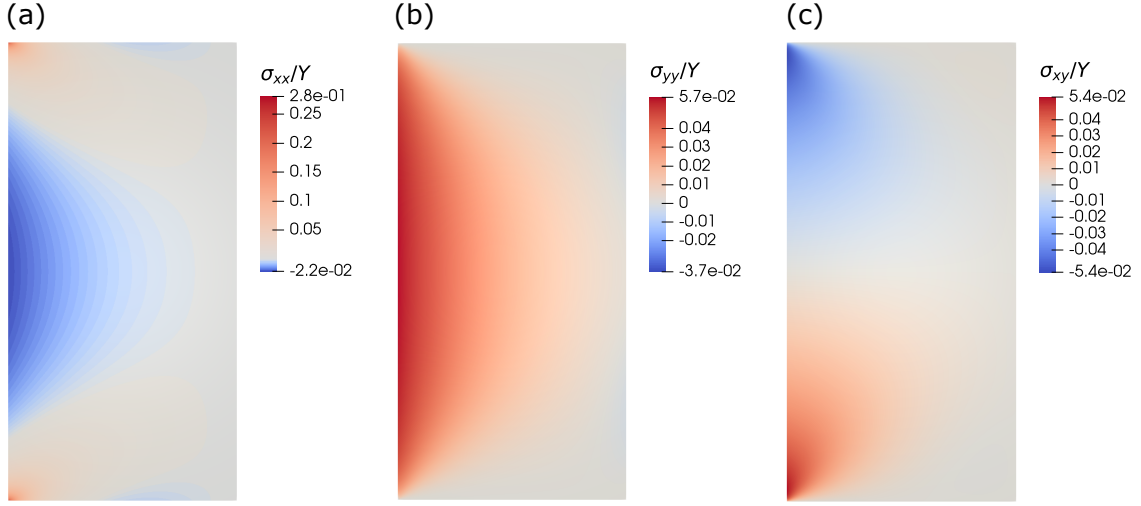

FIG. S1. In-plane stress fields for  $\sigma_{xx}/Y$ ,  $\sigma_{yy}/Y$  and  $\sigma_{xy}/Y$  from FEniCS calculation.

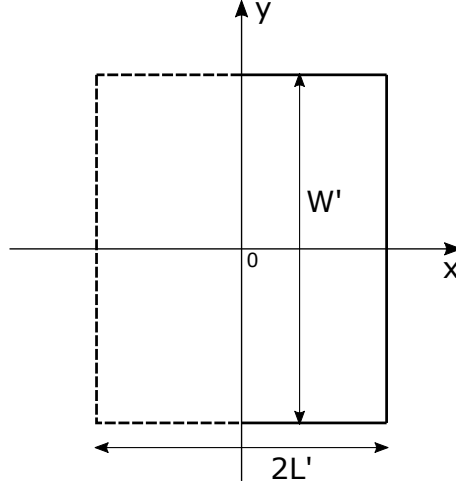

FIG. S2. The doubled system. The original elastic sheet in  $x \geq 0$  is doubled by reflection about the  $y$  axis.

close to the clamping is a key feature of the stress fields, regardless of the aspect ratio of the sheet.  $\sigma_{xy}$  is symmetric about the  $x$  axis but with opposite sign, as expected.

#### IV. ANALYTIC CALCULATION OF IN-PLANE STRESS

Taking the Hookean approximation and suppressing any out of plane displacement, the in-plane stress fields satisfy [15]

$$\partial_i \sigma_{ij} = 0. \quad (\text{S3})$$

To solve this 2D elasticity problem with the Airy stress function technique, boundary conditions on all sides in terms of stresses are needed. The stress, specifically  $\sigma_{xx}$  due to clamping, is, however, unknown. Rather, the boundary condition at  $x = 0$  is given in terms of the displacement field – Eq. (3) in the main text. A way around this problem is to double the original system to the region  $-L' \leq x \leq L'$  and  $-W'/2 \leq y \leq W'/2$  by reflecting it along the  $y$  axis (see Fig. S2). In the doubled system, we no longer need to provide any condition at  $x = 0$  as it is now an internal edge. The condition  $u_x(x = 0, y) = 0$  is also satisfied automatically. We introduce the Airy stress function  $\chi$ , such that  $\sigma_{xx} = \chi_{,yy}$ ,  $\sigma_{yy} = \chi_{,xx}$ , and  $\sigma_{xy} = -\chi_{,xy}$ , where

the subscripts denote differentiation. Eq. (S3) implies that  $\chi$  is biharmonic:

$$\Delta^2 \chi = 0. \quad (\text{S4})$$

The most general solution involves an infinite series of products in trigonometric and hyperbolic functions in both  $x$  and  $y$ . To gain analytic tractability, we approximate the boundary conditions in two ways. First, instead of imposing a delta function localized at  $x = 0$  for  $\sigma_{yy}$  due to clamping, we impose a delocalized boundary condition  $\sigma_{yy}(x, \pm W'/2) = f \cos(\lambda x)$  on the top and bottom edges, where  $\lambda = \pi/2L'$ . Here  $f$  is a force density to be determined self-consistently. Second, we impose the weak boundary condition  $\int \sigma_{xy}(\pm L', y) dy = 0$  on the left and right edges, instead of the strong traction-free condition  $\sigma_{xy} = 0$ . We expect that the relaxation enabled by thermal fluctuations fully justifies these less stringent boundary conditions. The remaining boundary conditions are  $\sigma_{xx}(x = \pm L', y) = 0$  and  $\sigma_{xy}(x, y = \pm W'/2) = 0$ . Eq.(S3) can now be solved with the simple ansatz

$$\chi = [A \cosh(\lambda y) + B y \sinh(\lambda y)] \cos(\lambda x), \quad (\text{S5})$$

which is an even function in both  $x$  and  $y$ , since  $\sigma_{xx}$  and  $\sigma_{yy}$  should be even in both directions. If we keep more than one Fourier component in  $\sigma_{yy}(x, \pm W'/2)$ , then  $\chi$  will be a summation of similar functions with  $A \rightarrow A_n$ ,  $B \rightarrow B_n$ , and  $\lambda \rightarrow \lambda_n$ . The stress fields are given by

$$\begin{aligned} \sigma_{xx} &= \chi_{,yy} = [(A\lambda^2 + 2B\lambda) \cosh(\lambda y) + B\lambda^2 y \sinh(\lambda y)] \cos(\lambda x) \\ \sigma_{yy} &= \chi_{,xx} = (-\lambda^2) [A \cosh(\lambda y) + B y \sinh(\lambda y)] \cos(\lambda x) \\ \sigma_{xy} &= -\chi_{,xy} = [B\lambda y \cosh(\lambda y) + (A\lambda + B) \sinh(\lambda y)] \lambda \sin(\lambda x). \end{aligned} \quad (\text{S6})$$

Note that due to the choice of an anti-periodic Fourier series,  $\sigma_{xx}(x = \pm L', y) = 0$  on the left and right edges is automatically satisfied by the ansatz. The weak boundary condition on  $\sigma_{xy}$  on the left and right edges is also satisfied by symmetry. The two unknowns  $A$  and  $B$  can be solved using the two boundary conditions on the top and bottom edges  $\sigma_{xy}(x, y = W'/2) = 0$  and  $\sigma_{yy}(x, \pm W'/2) = f \cos(\lambda x)$ . The result is given by

$$\begin{aligned} \sigma_{xx} &= \frac{f}{D} \{ [\sinh(\pi\alpha/4) - (\pi\alpha/4) \cosh(\pi\alpha/4)] \cosh(\pi y/2L') + \frac{\pi}{2L'} \sinh(\pi\alpha/4) y \sinh(\pi y/2L') \} \cos(\pi x/2L') \\ \sigma_{yy} &= \frac{f}{D} \{ [(\pi\alpha/4) \cosh(\pi\alpha/4) + \sinh(\pi\alpha/4)] \cosh(\pi y/2L') - \frac{\pi}{2L'} \sinh(\pi\alpha/4) y \sinh(\pi y/2L') \} \cos(\pi x/2L') \\ \sigma_{xy} &= \frac{f}{D} \left[ \frac{\pi}{2L'} \sinh(\pi\alpha/4) y \cosh(\pi y/2L') - (\pi\alpha/4) \cosh(\pi\alpha/4) \sinh(\pi y/2L') \right] \sin(\pi x/2L'), \end{aligned} \quad (\text{S7})$$

where  $D = \lambda W'/2 + \cosh(W'\lambda/2) \sinh(W'\lambda/2)$  is a constant, and we have used the aspect ratio  $\alpha \equiv W'/L' = W_0/L_0$ . We now determine  $f$  with the condition

$$u_y(0, \frac{W'}{2}) = -u_y(0, -\frac{W'}{2}) = \frac{W_0 - W'}{2} \equiv \frac{\epsilon}{2} W_0. \quad (\text{S8})$$

Applying the stress strain relation  $u_{yy} = \frac{1}{Y_R}(\sigma_{yy} - \nu_R \sigma_{xx})$  at  $x = 0$ , we integrate the strain to obtain displacement, yielding

$$\frac{f}{D} = \frac{\epsilon \pi W_0 Y_R}{8L' \sinh^2(\pi\alpha/4)}, \quad (\text{S9})$$

which completes our calculation of the in-plane stress. One sees that  $\sigma_{xx}(x = 0)$  is negative at  $y = 0$  and positive near the top or bottom edge, as shown in Fig.S3. Similarly, applying  $u_{xx} = \frac{1}{Y_R}(\sigma_{xx} - \nu_R \sigma_{yy})$  at  $y = 0$  and integrating  $u_{xx}$ , we obtain the compression of the middle strip – Eq. (5) in the main text.

## V. EFFECTIVE 1D ENERGY OF MIDDLE STRIP

We now derive the effective 1D energy presented in the main text. For convenience, we drop all subscripts in the elastic moduli, with the assumption that they are all renormalized. We also drop the prime in  $L'$  so that here  $-L \leq x \leq L$ . Starting from the full 2D energy in Eq. (2) in the main text, we drop the  $y$  derivative and  $u_y$  to obtain an energy density (per width)

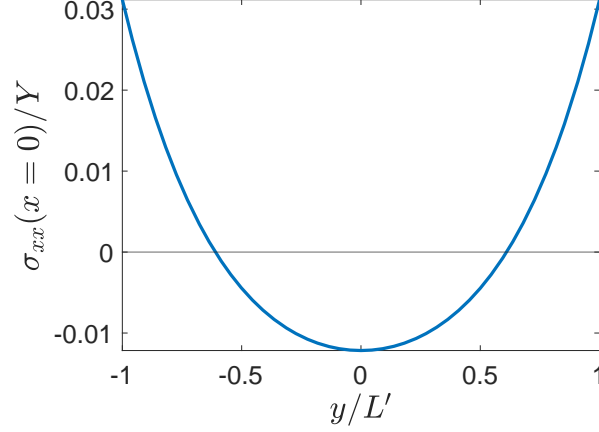

FIG. S3. Theoretical estimation of  $\sigma_{xx}$  at the clamp ( $x = 0$ ).  $\sigma_{xx} < 0$  in the middle and  $\sigma_{xx} > 0$  toward the top and bottom edges.

functional

$$\mathcal{E}[u_x, h] = \frac{\kappa}{2} \int dx \left( \frac{d^2 h}{dx^2} \right)^2 + \frac{Y}{2(1-\nu^2)} \int dx \left[ \frac{du_x}{dx} + \frac{1}{2} \left( \frac{dh}{dx} \right)^2 \right]^2 \equiv \mathcal{E}_b[u_x, h] + \mathcal{E}_s[u_x, h], \quad (\text{S10})$$

where we have used the identity  $2\mu + \lambda = \frac{Y}{1-\nu^2}$ .  $u_x$  is an odd function of  $x$  and satisfies the anti-periodic boundary condition  $u_x(-L) = -u_x(L) = \Delta/2$ . Following the established method (see e.g., Ref. [16, 17]), we define

$$A(x) \equiv \frac{1}{2} \left( \frac{dh}{dx} \right)^2. \quad (\text{S11})$$

To integrate out  $u_x$  and obtain an effective energy density for  $h$  only, we perform the Fourier series expansion for anti-periodic functions

$$\begin{aligned} u_x(x) &= \sum_{n=1} \sin(\lambda_n x) u_n \\ A(x) &= \sum_{n=1} \cos(\lambda_n x) A_n, \end{aligned} \quad (\text{S12})$$

where  $\lambda_n = \frac{(2n-1)\pi}{2L}$ . The boundary condition on  $u_x$  is equivalent to  $\sum_{n=1} (-1)^{n-1} u_n = -\Delta/2$ . The second term in Eq. (S10) in Fourier modes is

$$\mathcal{E}_s[u_x, h] = \frac{YL}{2(1-\nu^2)} \sum_{n=1} (\lambda_n u_n + A_n)^2. \quad (\text{S13})$$

Formally, the effective energy is then  $\mathcal{E}_{eff}[h] = \mathcal{E}_b - \log \left[ \int Du_x e^{-\mathcal{E}_s} \right]$ , with the appropriate boundary condition. We impose the boundary condition in the functional integral explicitly by introducing a delta function

$$\begin{aligned} \mathcal{E}_{eff}[h] &= \mathcal{E}_b - \log \left[ \int Du_x e^{-\mathcal{E}_s} \right] \\ &= \mathcal{E}_b - \log \left[ \int Du_x \delta[u_x(L) + \Delta/2] e^{-\mathcal{E}_s} \right] \\ &= \mathcal{E}_b - \log \left[ \int Du_x \int d\lambda e^{i\lambda[u_x(L) + \Delta/2] - \mathcal{E}_s} \right] \\ &= \mathcal{E}_b - \log \left[ \int d\lambda \int Du_x e^{i\lambda[\sum_{n=1} (-1)^{n-1} u_n + \Delta/2] - \mathcal{E}_s} \right]. \end{aligned} \quad (\text{S14})$$

The functional integral can be calculated in a straightforward way after a change of variable  $\lambda_n u_n + A_n \rightarrow u_n$ . Performing the remaining integral with respect to  $\lambda$  gives

$$\mathcal{E}_{eff}[h] = \mathcal{E}_b + \frac{Y}{L(1-\nu^2)} \left( \frac{\Delta}{2} + \sum_{n=1} (-1)^n \frac{A_n}{\lambda_n} \right)^2. \quad (\text{S15})$$

Now substituting  $A_n = \frac{1}{L} \int dx \frac{1}{2} \left( \frac{dh}{dx} \right)^2 \cos(\lambda_n x)$ , we observe that the above equation contains the Fourier series of a square-wave function. On the interval of interest  $-L \leq x \leq L$ , we have

$$\mathcal{E}_{eff}[h] = \frac{\kappa}{2} \int dx \left( \frac{d^2 h}{dx^2} \right)^2 + \frac{Y}{4L(1-\nu^2)} \left[ \Delta - \frac{1}{2} \int_{-L}^L dx \left( \frac{dh}{dx} \right)^2 \right]^2. \quad (\text{S16})$$

Eq. (7) presented in the main text is then obtained by dropping a constant term independent of  $h$ .

---

\* E-mail: bowick@kitp.ucsb.edu

- [1] L. D. Landau and E. M. Lifshitz, *Theory of Elasticity*, 3rd ed. (Butterworth-Heinemann, Singapore, 1999).
- [2] B. Audoly and Y. Pomeau, *Elasticity and Geometry* (Oxford University Press, Oxford, UK, 2010).
- [3] H. S. Seung and D. R. Nelson, *Phys. Rev. A* **38**, 1005 (1988).
- [4] J. Lidmar, L. Mirny, and D. R. Nelson, *Phys. Rev. E* **68**, 051910 (2003).
- [5] B. Schmidt and F. Fraternali, *J. Mech. Phys. Solids* **60**, 172 (2012).
- [6] D. Wan, D. R. Nelson, and M. J. Bowick, *Phys. Rev. B* **96**, 014106 (2017).
- [7] J. Glaser, T. D. Nguyen, J. A. Anderson, P. Lui, F. Spiga, J. A. Millan, D. C. Morse, and S. C. Glotzer, *Comput. Phys. Commun.* **192**, 97 (2015).
- [8] J. A. Anderson, J. Glaser, and S. C. Glotzer, *Computational Materials Science* **173**, 109363 (2020).
- [9] S. Plimpton, *J. Comput. Phys.* **117**, 1 (1995).
- [10] R. Nicklow, N. Wakabayashi, and H. G. Smith, *Phys. Rev. B* **5**, 4951 (1972).
- [11] A. Fasolino, J. H. Los, and M. I. Katsnelson, *Nat. Mater.* **6**, 858 (2007).
- [12] C. Lee, X. Wei, J. W. Kysar, and J. Hone, *Science* **321**, 385 (2008).
- [13] H. Zhao, K. Min, and N. R. Aluru, *Nano. Lett.* **9**, 3012 (2009).
- [14] A. Logg, K.-A. Mardal, and G. Wells, *Automated Solution of Differential Equations by the Finite Element Method: The FEniCS Book* (Springer Publishing Company, Incorporated, 2012).
- [15] L. Landau and E. Lifshitz, *Theory of Elasticity (Third Edition)* (Butterworth-Heinemann, 1986).
- [16] Nelson, D.R. and Peliti, L., *J. Phys. France* **48**, 1085 (1987).
- [17] A. Košmrlj and D. R. Nelson, *Phys. Rev. B* **93**, 125431 (2016).
